# Supplementary material for: Foundation Model based Open Vocabulary Task Planning and Executive System for General Purpose Service Robots
Source: arXiv:2308.03357 source file (2023-08-07)
Supplement: Supplementary file 1 [file appendix.tex]

% \section*{Appendix}
% \subsection{The Full Sentence of LLM Input used to Decompose Robot Commands into State Machines}
% Possible primitive tasks are [``move\_to'', ``visual\_question\_answering'', ``follow'', ``grasp'', ``pass\_to'', ``speak'', ``answer''] \\
% Q. Follow Robin from the couch to the corridor \\
% A. [[``move\_to'', ``the couch''], [``follow'', ``Robin''], [``move\_to'', ``the corridor'']] \\
% Q. Follow Charlie \\
% A. [[``follow'', ``Charlie'']] \\
% Q. Follow Robin to the bedroom \\
% A. [[``follow'', ``Robin''], [``move\_to'', ``the bedroom''] \\
% Q. Robot please meet Francis at the bed, follow her, and escort her back \\
% A. [[``move\_to'', ``the bed''], [``follow'', ``Francis'']] \\
% Q. Could you Tell me the gender of the person at the dishwasher \\
% A. [[``move\_to'', ``the dishwasher''], [``visual\_question\_answering'', ``what is the gender of the person ?'']] \\
% Q. Go to the dining room, find John at the table and answer his question. \\
% A. [[``move\_to'', ``the diningroom''], [``move\_to'', ``the table''], [``move\_to'', ``John''], [``answer'', ``question'']] \\
% Q. Robot please take the orange from the storage table and bring it to Alex at the couch \\
% A. [[``move\_to'', ``the storage table''], [``grasp'', ``the orange''], [``move\_to'', ``the couch''], [``move\_to'', ``Alex''], [``pass\_to'', ``Alex'']] \\
% Q. Bring me the object above the sponge from the desk \\
% A. [[``move\_to'', ``the desk''], [``move\_to'', ``the object above the sponge''], [``grasp'', ``the object above the sponge''], [``move\_to'', ``me''], [``pass\_to'', ``me'']] \\
% Q. Tell me how many cloth there are on the side table \\
% A. [[``move\_to'', ``the side table''], [``visual\_question\_answering'', ``how many cloth are on the side table ?'']] \\
% Q. Could you please meet Michael at the dining table, follow him, and escort him back \\
% A. [[``move\_to'', ``the dining table''], [``move\_to'', ``Michael''], [``follow'', ``Michael'']] \\
% Q. Navigate to the dishwasher, meet Robert, and lead him to the sink \\
% A. [[``move\_to'', ``the dishwasher''], [``move\_to'', ``Robert''], [``speak'', ``Please follow me.''], [``move\_to'', ``the sink'']] \\
% Q. Could you give drinks to all the elders in the living room \\
% A. [[``move\_to'', ``the living room''], [``move\_to'', ``drinks''], [``grasp'', ``drinks''], [``move\_to'', ``all the elders''], [``pass\_to'', ``all the elders'']] \\
% Q. Look for the fruits in the corridor \\
% A. [[``move\_to'', ``the corridor''], [``move\_to'', ``the fruits''], [``speak'', ``I found the fruits.'']] \\
% Q. Dump the garbage \\
% A. [[``move\_to'', ``the garbage''], [``grasp'', ``the garbage''], [``move\_to'', ``the trash''], [``pass\_to'', ``the trash'']] \\
% Q. Give me the left most object from the dining table \\
% A. [[``move\_to'', ``the dining table''], [``move\_to'', ``the left most object from the dining table'']] \\
% Q. Meet James at the bed, follow him, and go to the living room \\
% A. [[``move\_to'', ``the bed''], [``move\_to'', ``James''], [``follow'', ``James''], [``move\_to'', ``the living room'']] \\
% Q. Serve snacks to everyone in the bedroom \\
% A. [[``move\_to'', ``the bedroom''], [``move\_to'', ``snacks''], [``grasp'', ``snacks''], [``move\_to'', ``everyone''], [``pass\_to'', ``everyone'']] \\
% Q. Guide Alex from the entrance to the sink \\
% A. [[``move\_to'', ``the entrance''], [``move\_to'', ``Alex''], [``speak'', ``Please follow me.''], [``move\_to'', ``the sink'']] \\
% Q. Give me the biggest object from the cupboard \\
% A. [[``move\_to'', ``the cupboard''], [``move\_to'', ``the biggest object from the cupboard''], [``grasp'', ``the biggest object from the cupboard''], [``move\_to'', ``me''], [``pass\_to'', ``me'']] \\
% Q. Greet Charlie at the dishwasher and introduce it to Robert at the desk \\
% A. [[``move\_to'', ``the dishwasher''], [``move\_to'', ``Charlie''], [``speak'', ``Hello.''], [``speak'', ``Please follow me.''], [``move\_to'', ``the desk''], [``move\_to'', ``Robert''], [``speak'', ``This is Charlie'']] \\
% Q. Meet Robin at the bed, follow him, and navigate to the bedroom \\
% A. [[``move\_to'', ``the bed''], [``move\_to'', ``Robin''], [``follow'', ``Robin''], [``move\_to'', ``the bedroom'']] \\
% Q. Could you please escort Charlie to the sink \\
% A. [[``move\_to'', ``Charlie''], [``speak'', "Please follow me."], [``move\_to'', ``the sink'']] \\
% Q. Please tell me which are the three thinnest cutlery on the side table \\
% A. [[``move\_to'', ``Charlie''], [``speak'', "Please follow me."], [``move\_to'', ``the sink'']] \\
% Q. Please tell me which are the three thinnest cutlery on the side table \\
% A. [[``move\_to'', ``the side table''], [``visual\_question\_answering'', ``which are the three thinnest cutlery on the side table ?'']] \\
% Q. Tell me the pose of the person in the kitchen \\
% A. [[``move\_to'', ``the kitchen''], [``move\_to'', ``the person''], [``visual\_question\_answering'', ``What is the pose of the person ?'']] \\
% Q. Could you please locate the food in the living room \\
% A. [[``move\_to'', ``the living room''], [``visual\_question\_answering'', ``where is the food ?'']] \\
% Q. Go to the kitchen, find James at the sink and answer his question. \\
% A. [[``move\_to'', ``the kitchen''], [``move\_to'', ``the sink''], [``move\_to'', ``James''], [``answer'', ``question'']] \\
% Q. Could you face Francis at the exit and introduce it to Robin at the sink \\
% A. [[``move\_to'', ``the exit''], [``move\_to'', ``Francis''], [``speak'', ``Please follow me.''], [``move\_to'', ``the sink''], [``move\_to'', ``Robin''], [``speak'', ``This is Francis'']] \\
% Q. Look for the orange in the dining room \\
% A. [[``move\_to'', ``the dining room''], [``move\_to'', ``the orange''], [``speak'', ``I found the orange.'']] \\
% Q. Meet Francis and ask her what's your name \\
% A. [[``move\_to'', ``Francis''], [``speak'', ``what's your name'']] \\
% Please answer the below question as a nested python list without any decoration such as ``Answer: '' and ``A''. \\
